# Supplementary material for: Nonlinear Initialization Methods for Low-Rank Neural Networks
Source: arXiv:2202.00834 source file (2022-05-20)
Supplement: Supplementary file 1 [file appendix_empirical_gspectral_variants.tex]

\section{Appendix: More Empirical Variants of GSpectral}

\textbf{GSpectral with Orthogonal Regularization} Similarly to the spectral warm start, we can explicitly penalize deviations from orthogonality for the weights $U_i, V_i$ over the course of the GSpectral optimization procedure, by using either of the following metrics for orthogonality: 
\begin{definition}[Orthogonal Regularization for GSpectral]
We can penalize the weights $U \in \mathbb{R}^{n \times r}$ to encourage orthogonality by adding a constant times one of the following terms:
\begin{enumerate}
    \item $\ell_1$ Orthogonal Penalty: $\lambda \sum_{i \neq j}^n |U_i^TU_j|$
    \item $\ell_2$ Orthogonal Penalty: $\lambda \sum_{i \neq j}^n (U_i^TU_j)^2$
\end{enumerate}
where $U_i, U_j$ are rows of $U$.
Another important design choice in these penalties is whether or not to penalize the scale of the columns -- in particular, we may prefer to only ensure that correlations are close to zero. If we accept scale-invariance, we can penalize any matrix distance to the projection of the weights to the orthogonal manifold, which is given by 
\[
\textnormal{Proj}_{\mathcal{O}}\left(W\right) = UV^T
\]
where $W = U\Sigma V^T$ is the singular value decomposition.
\end{definition}
Orthogonality at initialization has been shown to be a desirable property of the weights for training neural networks in various settings [ADD CITATIONS HERE].
The Orthgonal-GSpectral approach has the advantage that we can tune the degree to which we are willying to trade off orthogonality and the value of the GSpectral objective, but pay a computational efficiency cost, since the resulting optimization is slower in practice.
