# Supplementary material for: Nonlinear Initialization Methods for Low-Rank Neural Networks
Source: arXiv:2202.00834 source file (2022-05-20)
Supplement: Supplementary file 2 [file appendix_experiments.tex]

\section{Appendix: Experiments}

\subsection{More Details on Main Experimental Setup} \label{subsec:experiment_setup_details}

\subsection{More Details on Downstream Generalization Experiment}

\subsection{More Experiment Analysis}

\subsection{More Results} \label{subsec:more_experiment_results}
